# Supplementary material for: A review on the charging station planning and fleet operation for electric freight vehicles
Source: arXiv:2311.16419 source file (2023-11-28)
Supplement: Supplementary file 1 [file benders.tex]

\section{Benders Decomposition Algorithm}\label{sec:benders_algo}

\begin{algorithm}[H]
\begin{algorithmic}[1]
\State Let $UB$ and $LB$ be upper bound and lower bound, respectively.
\State Initialization: $UB$ \gets +$\infty$
\State Solve the master problem: $LB \gets Objective\:Function$
\While{$UB-LB \geq 0.01$}
    \State Solve subproblem (SP)
    \If {SP is infeasible}
        \State Add slack variables to coupling constraints
        \State Augment the objective function with penalty multiplier with each slack variable
        \State Resolve the SP
    \EndIf
    \If {SP is feasible}
        \State Update $UB$. $UB:= min(current \:UB, \sum(objective\:value\:of\:SP\:and\:MP))$ 
        \State Find the dual of constraints of SP
        \State Add benders' (i.e., optimality) cut to MP
    \EndIf
    \State Solve MP
    \State Update $LB$:$LB \gets Objective\:Function$ 
\EndWhile
\caption{Pseudo-code for Benders' decomposition Algorithm}
\end{algorithmic}
\end{algorithm}
