# Supplementary material for: A review on the charging station planning and fleet operation for electric freight vehicles
Source: arXiv:2311.16419 source file (2023-11-28)
Supplement: Supplementary file 2 [file branch_and_cut.tex]

\section{Branch and Cut Algorithm}\label{sec:branch_and_cut_algo}

\begin{algorithm}[H]
\begin{algorithmic}[1]
\State Let $x^*$ is optimal solution and $v^*$ is the best objective value, respectively.
\State Initialization: $x^*$=null and $v^*$=+$\infty$
\State Add the initial MILP to $\mathcal{L}$, the set of active problems
\While{$\mathcal{L}$ is not empty}
    \State Select and remove (de-queue) a problem from $\mathcal{L}$
    \State Solve LP relaxation of the problem
    \If {The solution is infeasible}
        \State Go back to line 4
    \Else
        \State Denote the solution by $x$ with objective value $v$
    \EndIf
    \If {$v$ $\geq$ $v^*$}
        \State Go back to line 4
    \Else
        \If {$x$ is Integer}
            \State Set $v^*$ $\gets$ $v$ and $x^*$ $\gets$ $x$
            \State Go back to line 4
        \EndIf
    \EndIf
    \State Search for cutting planes that are violated by $x$
    \If {Cutting planes are found}
        \State Add them to the LP relaxation
            \State Go back to line 6
    \Else
        \State Branch to partition the problem into new problems with restricted feasible regions.
        \State Add these problems to $\mathcal{L}$ and go back to line 4
    \EndIf
\EndWhile
\State return $x^*$
\caption{Pseudo-code for Branch and Cut Algorithm}
\end{algorithmic}
\end{algorithm}
